# Supplementary material for: From Metadynamics to Dynamics
Source: arXiv:1309.5323 ancillary file (2013-12-05)
Supplement: Supplementary file 1 [file supplement_tiwary_parrinello.pdf]

# Supplemental Information to ‘From Metadynamics to Dynamics’

Pratyush Tiwary and Michele Parrinello

(Dated: September 20, 2013)

This supplement includes details of the simulation protocols employed in the main paper and plots that are further illustrative of the ideas presented there.

## I. 2-D MODEL POTENTIAL

In this section we provide details of the two-dimensional model potential which is the first example considered in the main text and was first introduced in Ref. [1]. This potential is periodic in the $x$-direction (periodicity of 3) and harmonic in $y$. The potential energy landscape is shown in Fig. 1(a) in the main text and is given by:

$$V(x, y) = cos(2\pi x)(1 + 4y) + \pi y^2 - 0.75cos(2\pi x/3) \tag{1}$$

To maintain the desired temperatures, we used a Langevin thermostat [2] with integration time step of 0.01, mass=1 and Langevin frequency of 0.5 (see [1] for details on units) at various temperatures between $1/(k_B T) = 5$ and 8. Well-tempered metadynamics [3] was used, with initial Gaussian height of 0.1 energy unit, width of 0.02 energy units squared and deposition stride of every $10^6$ integration steps. Various values of the bias factor in well-tempered metadynamics (see [3] for definition of bias factor) corresponding to effective temperatures of 0.75, 0.625 and 0.5, as well as various values of the initial Gaussian height and width were used to ascertain robustness of the proposed method. The kinetic Monte Carlo results were taken from [1].

The one-dimensional diffusion as reported in Fig. 1(b) in main manuscript was obtained from direct MD and from our approach using the time evolution of the mean squared displacement:

$$D = \frac{1}{2}\frac{d}{dt}\langle[x(t) - x(0)]^2\rangle \tag{2}$$

Fig. 1 shows a typical profile of the added bias after long times (i.e. after the diffusion constant has already converged to its values reported in the main text). As can be seen by comparing this figure to Fig. 1(a) in main text, following our recipe of infrequent bias deposition there was no bias added in the transition region for the higher pathway (transition region taken from Ref. [1]) even after it had been taken multiple times.

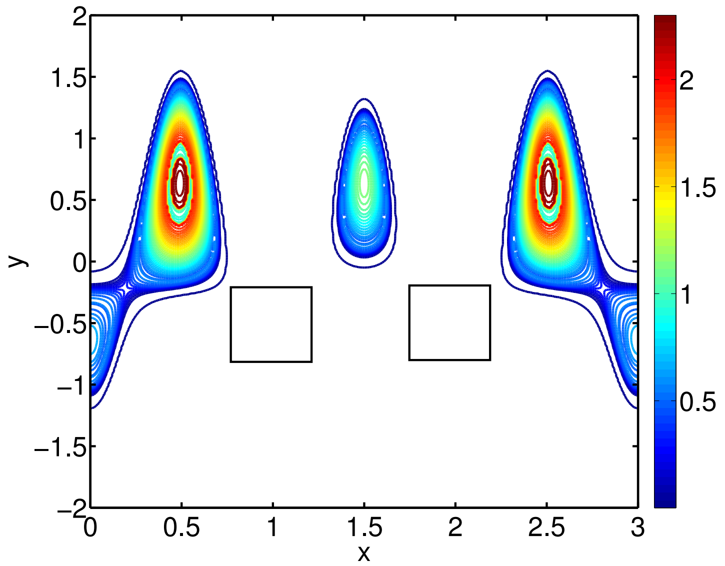


FIG. 1. A typical scenario for the deposited bias for the 2-d model potential (Eq. 1) after long times, showing how no bias was added in the transition state regions (black rectangular boxes) [1]. The lowest contour is at 0.02 energy unit.

## II. ALANINE DIPEPTIDE IN VACUUM

The second example we considered is the $C_{7eq} \rightarrow C_{7ax}$ conformational change in the alanine dipeptide molecule. These two stable states, differentiated by values of the backbone dihedral angles $(\Phi, \Psi)$ are separated by a barrier of $\approx$ 8 kcal/mol. Fig. 2(a) gives a ball and stick representation of the alanine dipeptide molecule with definitions of the relevant dihedral angles.

We used a Langevin thermostat to enforce the temperature [2], a time step of 0.2 fs, AMBER03 forcefield [7] and GROMACS4.5 molecular dynamics code patched with PLUMED [8, 9]. Well-tempered metadynamics was performed using $\Phi$ and $\Psi$ as CVs with bias factor of 11 at 200 K, and smaller bias factor at higher temperatures to keep roughly the same fictitious temperature $T + \Delta T$ of the CVs. The initial Gaussian height was 0.3 kcal/mol, the width was 0.25 rad for both CVs, and the deposition stride was 20 ps (compared to 0.12 ps used in Ref. [3] where free energy surface reconstruction was one of the objectives). A single alanine dipeptide molecule was kept in a periodic cubic box of edge 2.5$\mathring{A}$. The LINCS algorithm handled bond constraints [10] while the Particle-Mesh Ewald scheme was used

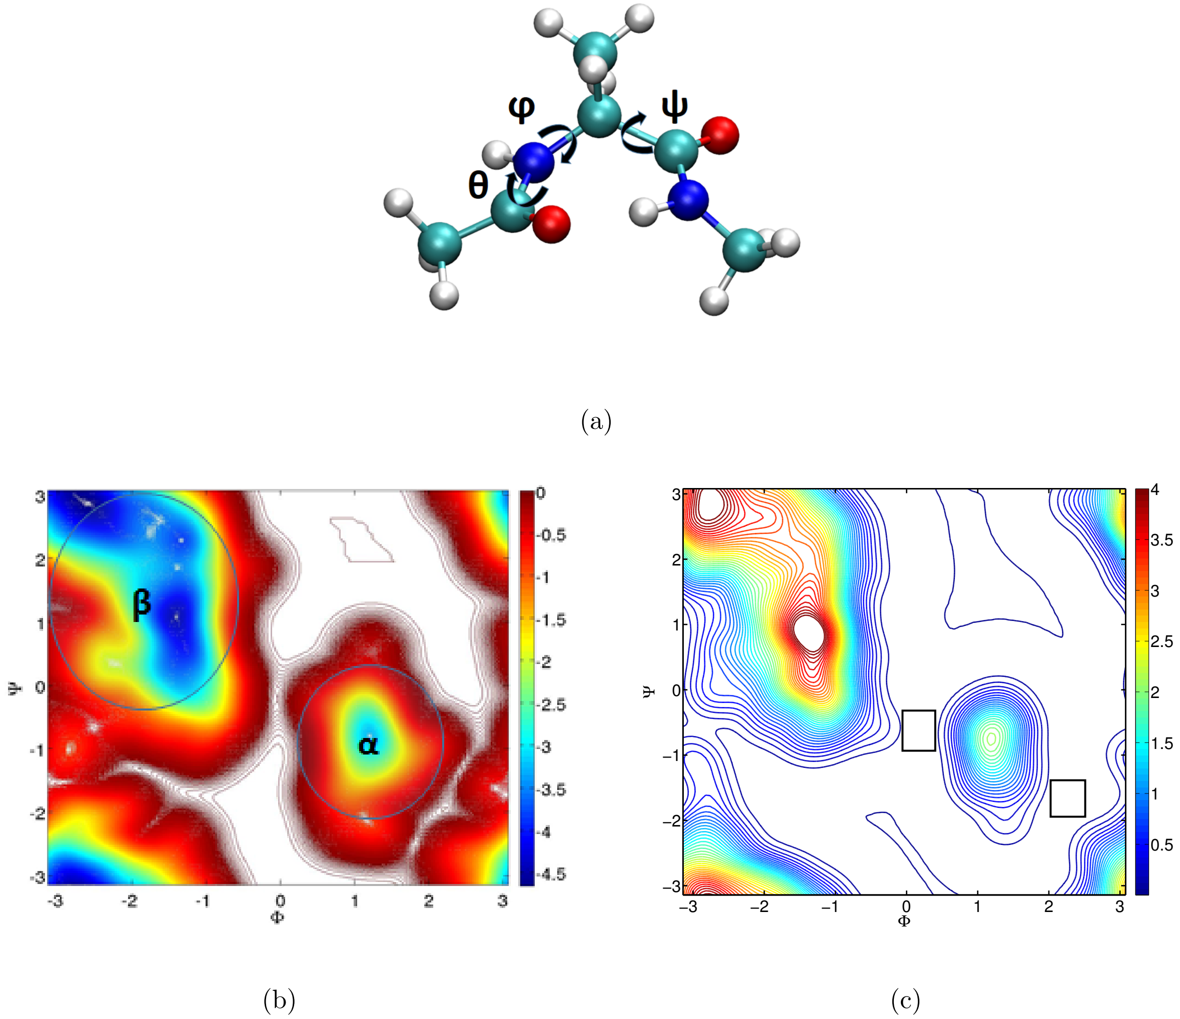


FIG. 2. (a)Ball and stick representation of the alanine dipeptide molecule with definitions of the relevant dihedral angles. 3 dihedral angles are marked: $\theta(O-C-N-C_\alpha)$, $\Phi(C-N-C_\alpha-C)$ and $\Psi(N-C_\alpha-C-N)$. The image has been constructed using VMD [4]. (b) Free energy surface in kcal/mol as a function of the two dihedral angles $\Phi$ and $\Psi$ obtained with well-tempered metadynamics, showing the two stable basins marked with blue ellipses. (c) Deposited bias in kcal/mol as a function of the two dihedral angles $\Phi$ and $\Psi$ obtained with well-tempered metadynamics with infrequent bias deposition at 300 K. The black rectangular boxes indicate the rough transition state regions as per Ref. [5]. It can be seen that no bias was added in these regions even after the metadynamics had visited both stable states multiple times. Contours are drawn every 0.1 kcal/mol.

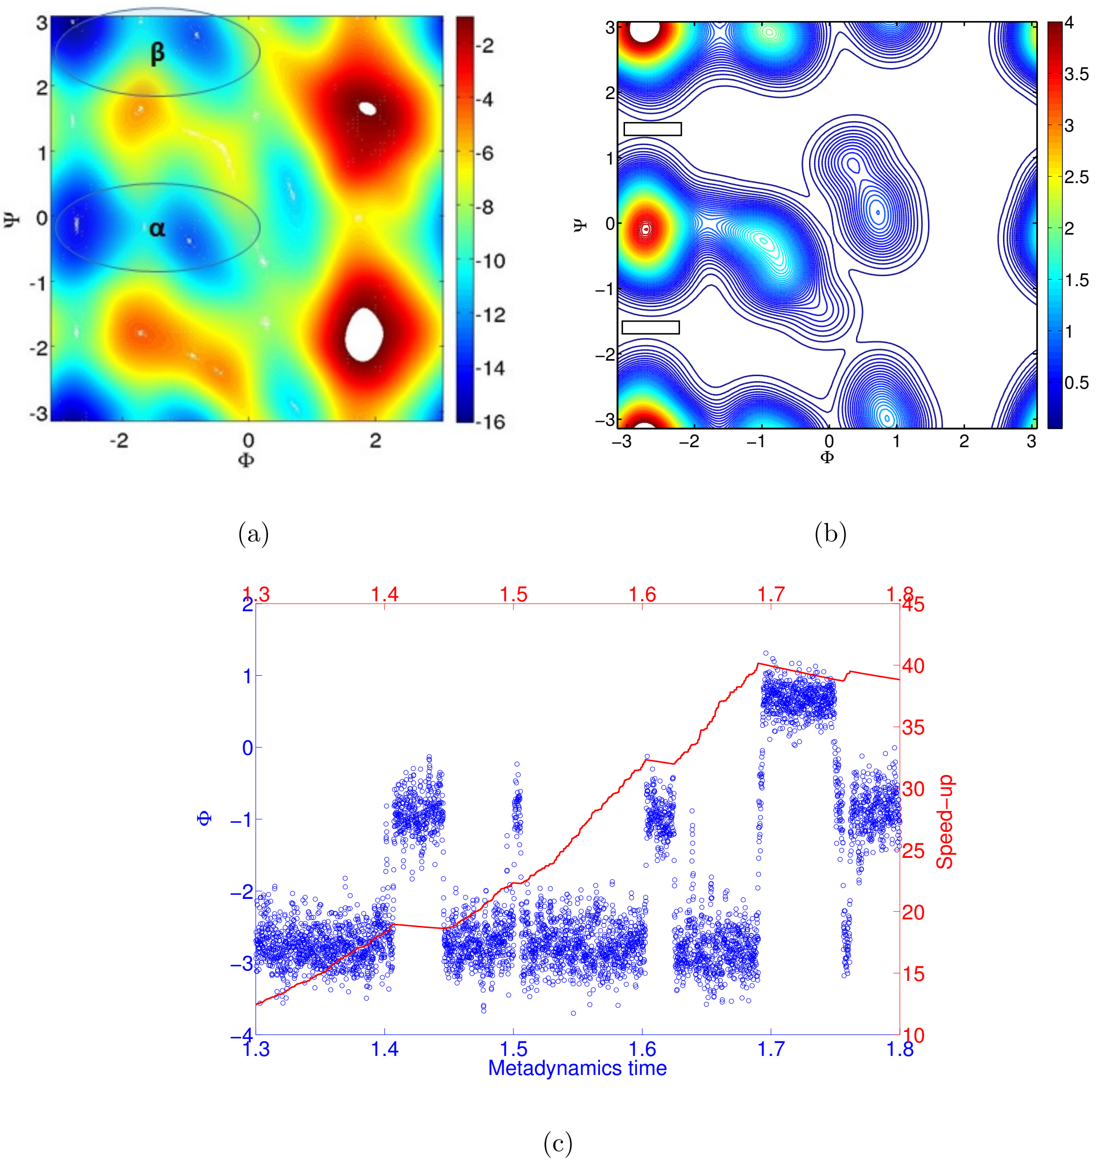


FIG. 3. (a) Free energy surface in kcal/mol for stiffened alanine dipeptide in water as a function of the two dihedral angles Φ and Ψ obtained with well-tempered metadynamics, showing the two stable basins marked with blue ellipses. (b) Deposited bias in kcal/mol as a function of the two dihedral angles Φ and Ψ obtained with well-tempered metadynamics with infrequent bias deposition at 300 K. The black rectangular boxes indicate the rough transition state regions as per Ref. [6]. It can be seen that no bias was added in these regions even after the metadynamics had visited both stable states multiple times. Contours are drawn every 0.05 kcal/mol.(c) Acceleration $\alpha$ versus metadynamics time (in ns) at 300 K overlaid with corresponding profile of dihedral angle Φ, showing kinks each time transition happens from one basin to another.

to treat long-distance electrostatic interactions [11]. The non-bonded van der Waals cut-off radius was 0.8 nm.

Fig. 2(b) shows the free energy surface for this molecule, along with the rough locations of the stable states. There is another shallow minimum next to the $C_{7eq}$ minimum, and we combine these two together in the $\beta$ basin as in Ref. [5] and several other works. In Fig. 2(c) we provide a typical profile of the deposited bias a function of the two dihedral angles after multiple conformational transitions, showing how no bias was deposited in the known transition state regions [5] for this system.

## III. STIFFENED ALANINE DIPEPTIDE IN WATER

We used a Langevin thermostat to enforce the temperature [2], time step of 1 fs, AMBER96 forcefield [7] and GROMACS4.5 molecular dynamics code patched with PLUMED [8, 9]. Well-tempered metadynamics was performed using $\Phi$ and $\Psi$ as CVs with bias factor of 10 at 300 K. The initial Gaussian height was 0.36 kcal/mol, the width was 0.3 rad for both CVs, and the deposition stride was 25 ps. A single alanine dipeptide molecule was solvated by 620 TIP3P water molecules [12] in a periodic cubic box of edge $2.93\AA$. The LINCS algorithm handled bond constraints [10] while the Particle-Mesh Ewald scheme was used to treat long-distance electrostatic interactions [11]. The non-bonded van der Waals cut-off radius was 0.8 nm.

Since the actual alanine dipeptide in water system has a barrier between its two main basins of only around 2 kcal/mol [6], the transitions in that system can easily be sampled using ordinary unbiased molecular dynamics, and no enhanced sampling scheme is needed. Thus in order to analyze if our method works in a true rare event system in the presence of a fluctuating environment, we stiffened the terms in the force field for the dihedral angles $\Phi$ and $\Psi$(Fig. 2 (a)) by changing the corresponding entry in the GROMACS topology file. Fig. 3(a) shows the free energy surface for this molecule in water, along with the rough locations of the stable conformations. In Fig. 3(b) we provide a typical profile of the deposited bias a function of the two dihedral angles after multiple conformational transitions, showing how no bias was deposited in the known transition state regions [6] for this system. In Fig. 3(c) we show a section of the acceleration versus metadynamics time profile for this system, overlaid with the corresponding profile in dihedral angle $\Phi$. Just like as in Fig. 2(c) in the

main text for alanine dipeptide in vacuum, we find kinks in this plot each time the system crosses from one stable basin to another.

---


[1] A. F. Voter *J. Chem. Phys.*, vol. 106, no. 11, pp. 4665–4677, 1997.

[2] G. Bussi, D. Donadio, and M. Parrinello, "Canonical sampling through velocity rescaling," *J. Chem. Phys.*, vol. 126, no. 1, pp. 014101–014101, 2007.

[3] A. Barducci, G. Bussi, and M. Parrinello *Phys. Rev. Lett.*, vol. 100, no. 2, p. 020603, 2008.

[4] W. Humphrey, A. Dalke, and K. Schulten *Journal of molecular graphics*, vol. 14, no. 1, pp. 33–38, 1996.

[5] P. G. Bolhuis, C. Dellago, and D. Chandler *Proc. Nat. Acad. Sci.*, vol. 97, no. 11, pp. 5877–5882, 2000.

[6] W.-N. Du, K. A. Marino, and P. G. Bolhuis *J. Chem. Phys.*, vol. 135, p. 145102, 2011.

[7] D. A. Case, T. E. Cheatham, T. Darden, H. Gohlke, R. Luo, K. M. Merz, A. Onufriev, C. Simmerling, B. Wang, and R. J. Woods *J. Comp. Chem.*, vol. 26, pp. 1668–1688, 2005.

[8] E. Lindahl, B. Hess, and D. Van Der Spoel *J Mol. Model.*, vol. 7, no. 8, pp. 306–317, 2001.

[9] M. Bonomi, D. Branduardi, G. Bussi, C. Camilloni, D. Provasi, P. Raiteri, D. Donadio, F. Marinelli, F. Pietrucci, R. A. Broglia, *et al. Comp. Phys. Comm.*, vol. 180, no. 10, pp. 1961–1972, 2009.

[10] B. Hess, H. Bekker, H. J. Berendsen, and J. G. Fraaije *J. Comp. Chem.*, vol. 18, no. 12, pp. 1463–1472, 1997.

[11] T. Darden, D. York, and L. Pedersen *J. Chem. Phy.*, vol. 98, p. 10089, 1993.

[12] W. L. Jorgensen, J. Chandrasekhar, J. D. Madura, R. W. Impey, and M. L. Klein *J. Chem. Phy.*, vol. 79, p. 926, 1983.
